# Supplementary material for: Rethinking Video with a Universal Event-Based Representation
Source: arXiv:2408.06248 source file (2024-08-12)
Supplement: Supplementary file 1 [file appendix.tex]

\clearpage
\phantomsection

{\def\chapter*#1{} % suppress bibliograph header.

\addcontentsline{toc}{chapter}{APPENDIX}
\begin{center}
% Don't use \Large to keep the graduate school from getting mad.
\textbf{APPENDIX}
%\vspace{11pt}
\end{center}

Appendix here...
